# Supplementary material for: Approximation Algorithms for Multi-Robot Patrol-Scheduling with Min-Max Latency
Source: arXiv:2005.02530 source file (2020-07-14)
Supplement: Supplementary file 1 [file 1D_appendix.tex]

\section{Exact Algorithms for Sites of Uniform Weights in $\Reals^1$}\label{sec:1D_appendix}
\begin{theorem}\label{thm:1d-k1}
For a single robot ($k$=1) and $n$ sites in $\Reals^1$ of possibly different weights, there exists an optimal solution which is a simple zigzag. 
\end{theorem}
\begin{proof}
Let $s$ be the site maximizing $d_s w_{s}$, where $d_s$ denotes the distance to the furthest (end-)point from $s$. A simple zigzag schedule has maximum weighted latency $L = 2 d_s w_{s}$. 

Let $s'$ be the endpoint at distance $d_s$ from $s$. Any schedule has to visit $s'$ at some time $t' > L$. The last visit to $s$ before $t'$, cannot have happened after $t'- d_s$, since $d_s$ is the minimum time to get from $s$ to $s'$ (assuming unit speeds). Likewise the next visit to $s$ cannot before $t' + d_s$. Thus, the time between these two visits to $s$ is at least $2 d_s w_{s}$. Therefore, any schedule has maximum weighted latency at least $L$. Thus, a simple zigzag schedule is optimal.

% Assume the maximum latency of the optimal solution is $L$. In the optimal solution, the robot must visit the leftmost site $s_1$ and rightmost site $s_n$ at some time; otherwise $L=\infty$. 

% Now, take the next visit to the leftmost site $s_1$ after time $t_0>2L$, suppose it is at time $t_1$. 
% Every site is visited within time interval $[t_1-L, t_1)$ (and also in $[t_1, t_1+L)$). 
% For a site $s$, take the previous visit to $s$ before $t_1$, say at time $t_2$. $|t_1-t_2|\geq d(s, s_1)$. Similarly, take the next visit to $s$ after $t_1$, say at time $t_3$. $|t_3-t_1|\geq d(s, s_1)$. Thus the latency for $s$ is at least $2d(s, s_1)$. Similarly one can argue for a similar claim with respect to the rightmost site $s_n$.
% Thus $L \geq 2 d_s \cdot w_{s}$, where $d_s$ is the length from $s$ to the furthest endpoint.
% % , where $L_p$ is the length from $p$ to the furthest endpoint. 

% Now, look at the schedule of a simple zigzag, the maximum weighted latency is exactly $\max_{s\in P} 2 d_s w_{s}$. Thus, it is optimal.
\end{proof}

\begin{theorem}
%\label{lem: 1D_convert_to_disjoint}
\label{thm:1D_optimal}
For $k$ robots and $n\ge k$ sites in $\Reals^1$ of the same weight, there exists an optimal schedule such that each robot moves as a simple zigzag and all robots span disjoint intervals. 
\end{theorem}
\begin{proof}
%In $S$, every point is visited by at least one robot. Some robots may encounter each other in the running time. In the proof process, we mainly use the exchange argument to prove this lemma.
We first observe that we can assume that robots never meet: If two robots would meet at a location $q$ and cross paths, we could let them turn around and bounce back without affecting the latency of any site. Let $s$ be the leftmost site strictly to the right of $q$. The robot that comes from the right, does not need to move until it reaches $q$ but can already stop at $s$, without increasing the latency of any site. 

Thus, we can assume that robots do not meet, and that there is a strict left-to-right order on the robots. Let $r_1, \ldots, r_k$ be the robots in this order, and let $I_i = [a_i, b_i]$ be the interval visited by $r_i$. The strict order on the robots, also implies that $a_i < a_j$ for $i<j$, since $r_j$ cannot visit $a_i$ without meeting $r_i$.

We now argue inductively that the intervals $I_i$ are disjoint. Assume that all intervals to the left of $I_i$ are disjoint (and therefore, in particular do not include $a_i$). Since only $r_i$ visits $a_i$, the latency of $a_i$ is at least $2(b_i-a_i)$. A simple zigzag schedule achieves this latency for all sites in $I_i$ even without any help from other robots. Thus, 
there is no advantage in other robots visiting sites in $I_i$, and we can therefore assume that $I_i$ is disjoint from $I_j$ for $j>i$.

The argument assumes that if $i<k$, there are actually sites to the right of $I_i$. If this is not be the case, we can shorten previous intervals, and assign the remaining robots to one site each without increasing latency. Given that all $I_i$ are disjoint, we can schedule the robots independently. By Theorem~\ref{thm:1d-k1} a simple zigzag schedule is optimal for each of the robots.

\end{proof}

%By Lemma~\ref{lem: 1D_convert_to_disjoint}, 
%Now we have the following algorithm.

%\begin{theorem}
%\label{thm:1D_optimal}
%If all the weights are the same, there exists an optimal solution for $k$ robots is a set of $k$ disjoint zigzags, that cover the set $S$ by $k$ intervals with max length minimized.
%\end{theorem}

With Theorem~\ref{thm:1D_optimal}, the min-max latency problem reduces to the following: Given a set $S$ of $n$ numbers and a parameter $k$, compute the smallest $L$ such that $S$ can be covered by $k$ intervals of length at most $L$. When $S$ is stored in sorted order in an array, $L$ can be computed in $O(k^2 \log^2 n)$ time~\cite[Theorem 14]{abrahamsen2017range}. If $S$ is not sorted, there is an $\Omega (n \log n)$ lower bound in the algebraic computation tree model~\cite{ben1983lower}, since for $k=n-1$ element uniqueness reduces to this problem.

% we can use dynamic programming to find an optimal schedule. The subproblem $L(i, j)$ is defined as the maximum latency of using $j$ robots to cover the first $i$ sites, where $1\leq i\leq n$, and $1\leq j\leq k$. 
% There are $nk$ subproblems and each subproblem could be computed by using $O(n)$ other subproblems using the following recursive function: consider all possible values of $1\leq \ell\leq i-1$, the first $\ell$ sites are covered by using $j-1$ robots while the sites from $s_{\ell+1}$ to  $s_i$ are covered by one robot with a zigzag schedule,
% $$L(i, j)=\min_{1\leq \ell\leq i-1} \max \big (L(\ell, j-1), 2d(s_{\ell+1}, s_i)\big)$$
% The running time is $O(n^2k)$.
